# Supplementary material for: Improving Membership Inference in ASR Model Auditing with Perturbed Loss Features
Source: arXiv:2405.01207 source file (2024-05-02)
Supplement: Supplementary file 1 [file sectionX_appendix.tex]

\subsection{Sample level}
\begin{table*}[h]
    \centering
    \begin{tabular}{crrcc}
        \toprule
         \textbf{Feature Set} & \textbf{Accuracy} & \textbf{AUC} & \textbf{FPR = 0.1} & \textbf{FPR = 0.01} \\ \midrule

        All features & $ 85.62 \pm 0.11 $ & $ 92.64 \pm 0.11 $ & \begin{tabular}{lr}
            \textbf{AUC} & $ 73.22 \pm 0.44 $\\
            \textbf{FPR} & $ 9.99 \pm 0.23$\\
            \textbf{TPR} & $ 74.13 \pm 1.44 $\\
        \end{tabular} & \begin{tabular}{r}
            $ 54.92 \pm 1.24 $\\
            $ 1.02 \pm 0.11 $\\
            $ 19.07 \pm 3.14 $\\
        \end{tabular} \\ \midrule

        Error features & $ 70.05 \pm 0.22 $ & $ 77.28 \pm 0.17 $ & 
        \begin{tabular}{lr}
            \textbf{AUC} & $ 57.42 \pm 0.49 $\\
            \textbf{FPR} & $ 9.73 \pm 0.37  $\\
            \textbf{TPR} & $ 33.17 \pm 1.71 $\\
        \end{tabular} & \begin{tabular}{r}
            $ 51.27 \pm 0.48 $\\
            $ 0.97 \pm 0.17 $\\
            $ 5.56 \pm 1.49 $\\
        \end{tabular} \\ \midrule

        Loss features & $ 86.04 \pm 0.20 $ & $ 92.33 \pm 0.17 $ & 
        \begin{tabular}{lr}
            \textbf{AUC} & $ 71.08 \pm 0.78 $\\
            \textbf{FPR} & $ 10.01 \pm 0.17 $\\
            \textbf{TPR} & $ 75.15 \pm 1.36 $\\
        \end{tabular} & \begin{tabular}{r}
            $ 52.63 \pm 0.30 $\\
            $ 0.0 \pm 0.0 $\\
            $ 0.0 \pm 0.0 $\\
        \end{tabular} \\ \midrule

        Error + Loss features & $ 85.95 \pm 0.19 $ & $ 91.74 \pm 0.14 $ & \begin{tabular}{lr}
            \textbf{AUC} & $ 69.90 \pm 0.48 $\\
            \textbf{FPR} & $ 9.99 \pm 0.22 $\\
            \textbf{TPR} & $ 69.42 \pm 1.91 $\\
        \end{tabular} & \begin{tabular}{r}
            $ 53.37 \pm 0.48 $\\
            $ 0.47 \pm 0.39 $\\
            $ 7.55 \pm 6.19 $\\
        \end{tabular} \\ \midrule
        
        Loss feats. + Gauss. + Adv. & $ 86.55 \pm 0.14 $ & $ 93.02 \pm 0.11 $ & 
        \begin{tabular}{lr}
            \textbf{AUC} & $ 73.27 \pm 0.45 $\\
            \textbf{FPR} & $ 9.97 \pm 0.21 $\\
            \textbf{TPR} & $ 75.74 \pm 0.69 $\\
        \end{tabular} & \begin{tabular}{r}
            $ 53.57 \pm 0.64 $\\
            $ 0.82 \pm 0.40 $\\
            $ 12.77 \pm 6.55 $\\
        \end{tabular} \\
         \bottomrule
    
    \end{tabular}
    \caption{Per-feature results with random forest for LS-100 transformer on the sample level.}
    \label{tab:transLS100_sam_features}
\end{table*}
\begin{table*}[h]
    \centering
    \begin{tabular}{crrcc}
        \toprule
         \textbf{Feature Set} & \textbf{Accuracy} & \textbf{AUC} & \textbf{FPR = 0.1} & \textbf{FPR = 0.01} \\ \midrule

        All features & $41.05 \pm 4.04$ & $26.29 \pm 5.03$ & \begin{tabular}{lr}
            \textbf{AUC} & $47.83 \pm 0.52$\\
            \textbf{FPR} & $9.94 \pm 1.04$\\
            \textbf{TPR} & $1.68 \pm 1.73$\\
        \end{tabular} & \begin{tabular}{r}
            $49.81 \pm 0.12$\\
            $1.0 \pm 0.12$\\
            $0.29 \pm 0.45$\\
        \end{tabular} \\ \midrule

        Error features & $61.26 \pm 1.59$ & $67.67 \pm 1.87$ & 
        \begin{tabular}{lr}
            \textbf{AUC} & $53.81 \pm 0.66$\\
            \textbf{FPR} & $9.82 \pm 0.32$\\
            \textbf{TPR} & $22.14 \pm 1.39$\\
        \end{tabular} & \begin{tabular}{r}
            $50.56 \pm 0.33$\\
            $0.88 \pm 0.26$\\
            $2.63 \pm 1.04$\\
        \end{tabular} \\ \midrule

        Loss features & $57.02 \pm 0.56$ & $80.44 \pm 1.27$ & 
        \begin{tabular}{lr}
            \textbf{AUC} & $54.35 \pm 2.17$\\
            \textbf{FPR} & $9.16 \pm 0.88$\\
            \textbf{TPR} & $24.22 \pm 7.88$\\
        \end{tabular} & \begin{tabular}{r}
            $50.39 \pm 0.37$\\
            $0.00 \pm 0.00$\\
            $0.00 \pm 0.00$\\
        \end{tabular} \\ \midrule

        Error + Loss features & $66.28 \pm 1.52$ & $76.64 \pm 2.33$ & 
        \begin{tabular}{lr}
            \textbf{AUC} & $56.58 \pm 1.15$\\
            \textbf{FPR} & $9.86 \pm 0.62$\\
            \textbf{TPR} & $31.36 \pm 4.36$\\
        \end{tabular} & \begin{tabular}{r}
            $50.84 \pm 0.50$\\
            $0.83 \pm 0.36$\\
            $3.54 \pm 1.92$\\
        \end{tabular} \\ \midrule

        Loss feats. + Gauss. + Adv. & $69.83 \pm 1.74$ & $81.27 \pm 1.90$ & 
        \begin{tabular}{lr}
            \textbf{AUC} & $57.74 \pm 0.97$\\
            \textbf{FPR} & $9.92 \pm 0.92$\\
            \textbf{TPR} & $36.84 \pm 1.30$\\
        \end{tabular} & \begin{tabular}{r}
            $51.40 \pm 0.54$\\
            $0.93 \pm 0.12$\\
            $6.01 \pm 1.89$\\
        \end{tabular} \\ 
         \bottomrule
    
    \end{tabular}
    \caption{Per-feature results with random forest for LS-100 conformer on the sample level.}
    \label{tab:confLS100_sam_features}
\end{table*}

\subsection{Speaker level}
\begin{table*}[h]
    \centering
    \begin{tabular}{crrcc}
        \toprule
         \textbf{Feature Set} & \textbf{Accuracy} & \textbf{AUC} & \textbf{FPR = 0.1} & \textbf{FPR = 0.01} \\ \midrule
        All features & $ 77.66 \pm 0.21 $ & $ 83.69 \pm 0.22 $ & \begin{tabular}{lr}
            \textbf{AUC} & $ 68.15 \pm 0.50 $\\
            \textbf{FPR} & $ 9.95  \pm 0.12 $\\
            \textbf{TPR} & $ 61.44 \pm 1.07 $\\
        \end{tabular} & \begin{tabular}{r}
            $ 53.09 \pm 0.73 $\\
            $ 0.98  \pm 0.06 $\\
            $ 11.06 \pm 2.04 $\\
        \end{tabular} \\ \midrule

        Error features & $77.34 \pm 0.17$ & $82.24 \pm 0.22$ & 
        \begin{tabular}{lr}
            \textbf{AUC} & $ 62.64 \pm 0.60$\\
            \textbf{FPR} & $ 10.02 \pm 0.15$\\
            \textbf{TPR} & $ 51.67 \pm 1.57$\\
        \end{tabular} & \begin{tabular}{r}
            $ 52.49 \pm 0.49$\\
            $ 0.95  \pm 0.07$\\
            $ 9.11  \pm 1.02$\\
        \end{tabular} \\ \midrule

        Loss features & $ 76.01 \pm 0.27 $ & $ 81.26 \pm 0.15 $ & 
        \begin{tabular}{lr}
            \textbf{AUC} & $ 62.98 \pm 0.34 $\\
            \textbf{FPR} & $ 10.05 \pm 0.10 $\\
            \textbf{TPR} & $ 51.21 \pm 1.88 $\\
        \end{tabular} & \begin{tabular}{r}
            $ 51.84 \pm 0.48 $\\
            $ 0.93  \pm 0.20 $\\
            $ 7.76  \pm 1.31 $\\
        \end{tabular} \\ \midrule

        Error + Loss features & $ 77.18 \pm 0.19 $ & $ 82.49 \pm 0.16 $ & 
        \begin{tabular}{lr}
            \textbf{AUC} & $ 63.96 \pm 0.64 $\\
            \textbf{FPR} & $ 10.04 \pm 0.14 $\\
            \textbf{TPR} & $ 52.02 \pm 1.25 $\\
        \end{tabular} & \begin{tabular}{r}
            $ 53.55 \pm 0.73 $\\
            $ 1.02 \pm 0.10 $\\
            $ 11.68 \pm 1.95 $\\
        \end{tabular} \\ \midrule

        Loss feats. + Gauss. + Adv. & $ 78.31 \pm 0.23 $ & $ 83.89 \pm 0.13 $ & 
        \begin{tabular}{lr}
            \textbf{AUC} & $ 69.07 \pm 0.34 $\\
            \textbf{FPR} & $ 10.04 \pm 0.16 $\\
            \textbf{TPR} & $ 62.51 \pm 0.66 $\\
        \end{tabular} & \begin{tabular}{r}
            $ 53.12 \pm 0.47 $\\
            $ 0.92  \pm 0.12 $\\
            $ 11.77 \pm 2.27 $\\
        \end{tabular} \\
        \bottomrule
    \end{tabular}
    \caption{Per-feature results with random forest for LS-360 transformer on the speaker level.}
    \label{tab:transLS360_spk_features}
\end{table*}
\begin{table*}[h]
    \centering
    \begin{tabular}{crrcc}
        \toprule
         \textbf{Feature Set} & \textbf{Accuracy} & \textbf{AUC} & \textbf{FPR = 0.1} & \textbf{FPR = 0.01} \\ \midrule

        All features & $ 76.96 \pm 1.08 $ & $ 89.32 \pm 0.24 $ & \begin{tabular}{lr}
            \textbf{AUC} & $ 70.78 \pm 1.09 $\\
            \textbf{FPR} & $ 9.98 \pm 0.22 $\\
            \textbf{TPR} & $ 72.3 \pm 1.99 $\\
        \end{tabular} & \begin{tabular}{r}
            $ 53.93 \pm 0.52 $\\
            $ 0.98 \pm 0.06 $\\
            $ 13.98 \pm 2.25 $\\
        \end{tabular} \\ \midrule

        Error features & $ 82.78 \pm 0.23 $ & $ 89.31 \pm 0.16 $ & 
        \begin{tabular}{lr}
            \textbf{AUC} & $ 72.30 \pm 0.45 $\\
            \textbf{FPR} & $ 10.03 \pm 0.10 $\\
            \textbf{TPR} & $ 73.26 \pm 0.87 $\\
        \end{tabular} & \begin{tabular}{r}
            $ 53.88 \pm 0.66 $\\
            $ 0.95 \pm 0.08 $\\
            $ 16.35 \pm 2.44 $\\
        \end{tabular} \\ \midrule

        Loss features & $ 81.46 \pm 0.35 $ & $ 87.64 \pm 0.09 $ & 
        \begin{tabular}{lr}
            \textbf{AUC} & $ 69.75 \pm 0.44 $\\
            \textbf{FPR} & $ 9.99 \pm 0.13 $\\
            \textbf{TPR} & $ 67.86 \pm 1.59 $\\
        \end{tabular} & \begin{tabular}{r}
            $ 52.57 \pm 0.61 $\\
            $ 0.95 \pm 0.14 $\\
            $ 11.63 \pm 2.35 $\\
        \end{tabular} \\ \midrule

        Error + Loss features & $ 82.73 \pm 0.21 $ & $ 89.36 \pm 0.13 $ & \begin{tabular}{lr}
            \textbf{AUC} & $ 72.49 \pm 0.37 $\\
            \textbf{FPR} & $ 10.11 \pm 0.13 $\\
            \textbf{TPR} & $ 73.72 \pm 0.72 $\\
        \end{tabular} & \begin{tabular}{r}
            $ 55.26 \pm 1.12 $\\
            $ 0.98 \pm 0.09 $\\
            $ 20.20 \pm 2.94 $\\
        \end{tabular} \\ \midrule

        Loss feats. + Gauss. + Adv. & $ 84.13 \pm 0.17 $ & $ 90.76 \pm 0.18 $ & 
        \begin{tabular}{lr}
            \textbf{AUC} & $ 75.43 \pm 0.42 $\\
            \textbf{FPR} & $ 10.11 \pm 0.16 $\\
            \textbf{TPR} & $ 78.65 \pm 0.47 $\\
        \end{tabular} & \begin{tabular}{r}
            $ 54.05 \pm 0.74 $\\
            $ 0.97 \pm 0.05 $\\
            $ 18.45 \pm 3.24 $\\
        \end{tabular} \\
        
        \bottomrule
    
    \end{tabular}
    \caption{Per-feature results with random forest for LS-100 transformer on the speaker level.}
    \label{tab:transLS100_spk_features}
\end{table*}
\begin{table*}[h]
    \centering
    \begin{tabular}{crrcc}
        \toprule
         \textbf{Feature Set} & \textbf{Accuracy} & \textbf{AUC} & \textbf{FPR = 0.1} & \textbf{FPR = 0.01} \\ \midrule

        All features & $58.6 \pm 10.38$ & $67.85 \pm 8.11$ & \begin{tabular}{lr}
            \textbf{AUC} & $50.76 \pm 4.39$\\
            \textbf{FPR} & $10.07 \pm 1.16$\\
            \textbf{TPR} & $13.21 \pm 14.92!!!!!!!!! $\\ %(is the +- 14.92 correct?)
        \end{tabular} & \begin{tabular}{r}
            $50.03 \pm 0.53$\\
            $1.03 \pm 0.22$\\
            $1.26 \pm 2.26$\\
        \end{tabular} \\ \midrule

        Error features & $77.95 \pm 2.45$ & $86.65 \pm 1.43$ & 
        \begin{tabular}{lr}
            \textbf{AUC} & $65.94 \pm 1.69$\\
            \textbf{FPR} & $9.78 \pm 0.51$\\
            \textbf{TPR} & $54.71 \pm 5.89$\\
        \end{tabular} & \begin{tabular}{r}
            $52.89 \pm 0.85$\\
            $0.96 \pm 0.12$\\
            $10.93 \pm 2.59$\\
        \end{tabular} \\ \midrule

        Loss features & $82.62 \pm 0.80$ & $88.22 \pm 0.35$ & 
        \begin{tabular}{lr}
            \textbf{AUC} & $64.32 \pm 0.68$\\
            \textbf{FPR} & $10.02 \pm 0.06$\\
            \textbf{TPR} & $62.54 \pm 2.56$\\
        \end{tabular} & \begin{tabular}{r}
            $50.87 \pm 0.51$\\
            $0.97 \pm 0.11$\\
            $4.88 \pm 1.80$\\
        \end{tabular} \\ \midrule

        Error + Loss features & $77.54 \pm 2.49$ & $86.48 \pm 2.32$ & \begin{tabular}{lr}
            \textbf{AUC} & $64.82 \pm 3.69$\\
            \textbf{FPR} & $9.94 \pm 0.33$\\
            \textbf{TPR} & $53.34 \pm 9.58$\\
        \end{tabular} & \begin{tabular}{r}
            $52.83 \pm 1.23$\\
            $0.90 \pm 0.15$\\
            $10.08 \pm 3.94$\\
        \end{tabular} \\ \midrule

        Loss feats. + Gauss. + Adv. & $67.22 \pm 3.62$ & $81.62 \pm 2.99$ & 
        \begin{tabular}{lr}
            \textbf{AUC} & $62.72 \pm 2.87$\\
            \textbf{FPR} & $9.97 \pm 0.51$\\
            \textbf{TPR} & $43.67 \pm 7.81$\\
        \end{tabular} & \begin{tabular}{r}
            $52.59 \pm 0.72$\\
            $0.96 \pm 0.08$\\
            $10.99 \pm 2.40$\\
        \end{tabular} \\ 
        \bottomrule
    
    \end{tabular}
    \caption{Per-feature results with random forest LS-100 conformer on the speaker level.}
    \label{tab:my_label}
\end{table*}
\newpage
